# Supplementary material for: Measurements of differential charged-current cross sections on argon for electron neutrinos with final-state protons in MicroBooNE
Source: arXiv:2511.17342 source file (2026-03-05)
Supplement: Supplementary file 1 [file preamble_supplemental.tex]

% \RequirePackage{lineno} 

\documentclass[
 reprint,
 superscriptaddress,
%groupedaddress,
%unsortedaddress,
%runinaddress,
%frontmatterverbose, 
%preprint,
preprintnumbers,
%nofootinbib,
%nobibnotes,
%bibnotes,
 amsmath,amssymb,
 aps,
 prd,
 onecolumn
]{revtex4-2}

\usepackage{multirow}
\usepackage{gensymb}
\usepackage{svg}
\usepackage[caption=false]{subfig}
\usepackage{graphicx}
\usepackage{dcolumn}
\usepackage{lineno}
\usepackage{bm} 
\usepackage{amssymb}  
\usepackage{tikz}
\usepackage{hyperref}

\hypersetup{
    colorlinks=true,
    linkcolor=purple,
    filecolor=purple,      
    urlcolor=purple, 
    citecolor=purple
    }

\hyphenation{ALPGEN}
\hyphenation{EVTGEN}
\hyphenation{PYTHIA}
\hyphenation{Micro-BooNE}

\newcommand{\code}[1]{\texttt{#1}}
\newcommand{\pizero}{$\pi^0$}
\newcommand{\nue}{$\nu_{e}$}
\newcommand{\nuecc}{$\nu_{e}$ CC}
\newcommand{\nuebar}{$\bar{\nu}_{e}$}
\newcommand{\nuebarcc}{$\bar{\nu}_{e} CC$}
\newcommand{\numu}{$\nu_{\mu}$}
\newcommand{\numucc}{$\nu_{\mu} CC$}
\newcommand{\numubar}{$\bar{\nu}_{\mu}$}
\newcommand{\numubarcc}{$\bar{\nu}_{\mu} CC$}
\newcommand{\ppfx}{\code{PPFX}}
\newcommand{\npsel}{CC 1e0$\pi$Np}
